# Supplementary material for: Rethinking Targeted Adversarial Attacks For Neural Machine Translation
Source: arXiv:2407.05319 source file (2024-07-07)
Supplement: Supplementary file 1 [file appendix.tex]

\section{TWGA Algorithm}
\label{appendix:twga}
Algorithm~\ref{alg:adversarial example generation} illustrates the attacking process of TWGA.

\section{Details Regarding Pre-Trained Language Models}
\label{appendix: language models}
In \sref{para:objective}, we mention that we pre-trained two language models to calculate the fluency constraints in our objective function. Here we detail the training process as well as all the results related to these two models.

These two language models are trained on the WikiText-103 corpus~\cite{merity2016pointer} under the default training setting provided by Fairseq's language modeling task \footnote{\url{https://github.com/pytorch/fairseq/blob/main/examples/language_model/README.md}}. Noting that when training the right-to-left language model, we first manually reverse all the sentences of the WikiText-103 dataset, then train the model on this reversed dataset. The left-to-right and right-to-left language models achieve perplexity scores of 16.61 and 18.89 on the test set respectively, which indicates high model qualities.
\iffalse
\section{Manual Requirements for Substituting Tokens}
\label{appendix: manual requirements}
The following requirements are applied to determine whether a token sampled from the optimized adversarial distribution $\Gamma$ is eligible for substituting the original token or not.
\begin{itemize}[wide=0\parindent,noitemsep,topsep=0em]
%\setlength{\itemsep}{0.5pt}
%\setlength{\parsep}{0.5pt}
%\setlength{\parskip}{0.5pt}
    %\item This token should be in the source vocabulary $\mathbf{V}^{src}$.
    \item If the BPE signal `@@' appears in the original token, the newly sampled token should also contain this signal and vice versa.
    \item Both the original token and the sampled token are cased or uncased.
    \item The frequency of the sampled token in $\mathbf{V}^{src}$ is higher than 2000.
\end{itemize}
\fi
\section{Detailed Configuration}
\label{appendix:config}
Here we provide a detailed description of our configuration settings in the paper for training the NMT systems and implementing our targeted attack TWGA. 

\paragraph{TWGA.} 
When optimizing the adversarial distribution $\hat{\Gamma}$, we use the Adam optimizer \cite{kingma2014adam} with a learning rate of 3e-3. The batch size is set to 1 for 50 iterations, and we early stop the iteration when the adversarial loss $\mathcal{L}_{\text{adv}}$ reaches 0. When initializing $\Gamma$, the constant $\epsilon$ is set to 12. The margin $\mu$ in the adversarial loss is set to 3. %and the score threshold $\epsilon$ in the overlapped score match is 0.5. 
$\lambda_{1}$ and $\lambda_{2}$ in the objective function $\mathcal{L}$ are both set to 1. 

\paragraph{Training NMT Systems.}  We train both LSTM and TF for 300K steps with 6K warmup steps using the cosine learning rate scheduling strategy. During training, we use the Adam optimizer ($\beta_1=0.9, \beta_2=0.98)$ with a learning rate of 1e-4. Dropout rate is set to 0.3 and label smoothing rate is set to 0.2. The maximum number of tokens in a batch is set to 65536. 
All of our experiments are implemented with PyTorch \footnote{\url{https://pytorch.org/}} and Fairseq \footnote{\url{https://github.com/pytorch/fairseq}}.% with NVIDIA RTX3090 GPUs.

\begin{savenotes}
\begin{algorithm}[tb]

	\caption{Adversarial Example Generation}
	\label{alg:adversarial example generation}
	  %\algsetup{linenosize=\small}
	  \small
	\begin{algorithmic}[1]
		\REQUIRE a source sentence $\boldsymbol{x}$ with its targeted word $z$, set $\{\mathbf{Z}\}$ that contains all the reference translations of $z$. 
		\ENSURE An adversarial example $\boldsymbol{x'}$ for $\boldsymbol{x}$. 
		\STATE Initialize a probability matrix $\mathbf{P}$ from $\boldsymbol{x}$.
		\STATE $\Gamma$ $\longleftarrow$ Gumbel-softmax($\mathbf{P}$).
		\STATE At each decoding step, calculate $\mathcal{L_{\text{adv}}}$. Sum them up to get $\mathcal{L}$ after decoding.
		%\STATE Compute $\mathcal{L}$ with $e(\Gamma)$, $\mathbf{N}^t$ and $\mathcal{M}$ by Eq.\ref{new adv objective}.
		\STATE Optimize $\mathbf{P}$ with $\mathcal{L}$ by Eq.\ref{new adv objective}.
		\STATE num $\longleftarrow$ 0
		\WHILE{num < 100}
		\STATE $\Gamma$ $\longleftarrow$ Gumbel-softmax($\mathbf{P}$).
		\STATE Perturb $\boldsymbol{x}$ to $\boldsymbol{x'}$ using $\Gamma$.
		\IF {$\boldsymbol{x'}$ is an adversarial example for $\boldsymbol{x}$}
				\STATE \textbf{return} $\boldsymbol{x'}$.
		\ELSE
		\STATE num $\longleftarrow$ num $+$ 1
		\ENDIF
		\ENDWHILE
	\end{algorithmic}  
\end{algorithm}
\end{savenotes}

\iffalse
\section{Statistics of the Evaluation Set}
\label{appendix:statistics}
\tref{tab:statistics} lists the statistics of evaluation sets used in our experiments in~\sref{exp}.
\begin{table}[tb]

  \centering
   \setlength{\tabcolsep}{2mm}{
    %\resizebox{0.8\textwidth}{!!}
    \small
    \begin{tabular}{cccc}
    \toprule[1pt]
    &
      \textbf{Evaluation Set} & \textbf{\#Example} 
      & \textbf{Avg.Length}
      \\
     \midrule[0.5pt]
     LSTM &WMT & 2311&36.67   
     \\
     
     \midrule[0.5pt]
     \multirowcell{2}{$\text{TF}$} &
      WMT & 2263&36.16  \\
      ~&Para & 53834 & 22.94   \\
     \bottomrule[1pt]
    \end{tabular}
  }  
  %}  
    \caption{Statistics of the constructed evaluation sets.}% Avg.Len denotes the averaged length of source sequences in an evaluation set.}
  \label{tab:statistics}
\end{table}
\fi
\begin{table}[tb]

  \centering
   \setlength{\tabcolsep}{2.2mm}{
    %\resizebox{0.8\textwidth}{!!}
    \small
    \begin{tabular}{llccc}
    \toprule[1pt]
     & %\textbf{Method}
     & \textbf{Succ}$\uparrow$ 
      & \textbf{Edit} $\downarrow$ 
      %&  \textbf{PPL} $\downarrow$ 
      & \textbf{Query} $\downarrow$ 
      \\
     \midrule[0.5pt]
     \multirowcell{2}{$\text{LSTM}$}& Before
     & 57.68
     & 14.21
     & 226.71
     \\
     ~& After
     & 59.37
     & 19.56
     & 38.03 \\
     \midrule[0.5pt]
     \multirowcell{2}{$\text{TF}$} & Before
     & 47.19
     & 14.62
     & 263.86
     \\
     ~& After
     & 41.27
     & 19.02
     & 54.77 \\
     \bottomrule[1pt]
    \end{tabular}
  }  
  %}  
    \caption{Attacking results of Seq2Sick on WMT before/after we reduce its query number. Succ/Edit are reported by percentage (\%).}
  \label{tab:seq2sick}
\end{table}

\section{Human evaluation instructions.}
\label{appendix:human}
In this section, we provide the complete instructions on the three-point scoring scales mentioned in~\sref{meaningfulness}:
\begin{itemize}
    \item This adversarial example has more than 3 typos/grammatical errors. Or it is not fluent and complete. (1-meaningless)
\item This adversarial example has fewer than 3 typos/grammatical errors, and is fluent and complete. (2-mediocre)
\item This adversarial example is fluent and complete, and does not have grammatical mistakes. (3-meaningful)
\end{itemize}

\section{Implementing Baseline Attacks on Para.}
\label{appendix:seq2sick}
In \sref{attack results on para}, we also implement RR and the second strongest attack method on WMT (Seq2Sick) on Para for comparison. Since the size of Para is much larger than WMT, we modify the original implementation of Seq2Sick to make its Query value on a par with TWGA and thus becomes efficient enough to be applied on Para. To be specific, we not only reduce the number of iterations of Seq2Sick from 200 to 50 but also add an early-stopping module to stop the iteration when its adversarial loss reaches zero. \tref{tab:seq2sick} lists the attacking performances of Seq2sick on WMT before and after we reduce its number of queries. We can see that with less number of queries, Seq2Sick can still achieve similar Succ scores compared to its original implementation, though more tokens need to be modified for crafting an adversarial example. Overall, the Query-reduced version of Seq2Sick can provide good approximations of Seq2Sick's attacking results while enhancing the attack efficiency. Hence, we apply the Query-reduced version of Seq2Sick on Para to obtain attacking results.

\section{Example Case of Attacking a Verb with TWGA}
\label{appendix:case study}
In this section, we provides a case study of TWGA on attacking a verb.
As can be seen, TF fails to translate \textit{``offered''} in \fref{fig:pos examples} when TWGA attaches this targeted word to the newly added object \textit{``surveillance''} instead of the original \textit{``course''}.

\begin{figure}
    \centering
    \includegraphics[width=0.48\textwidth]{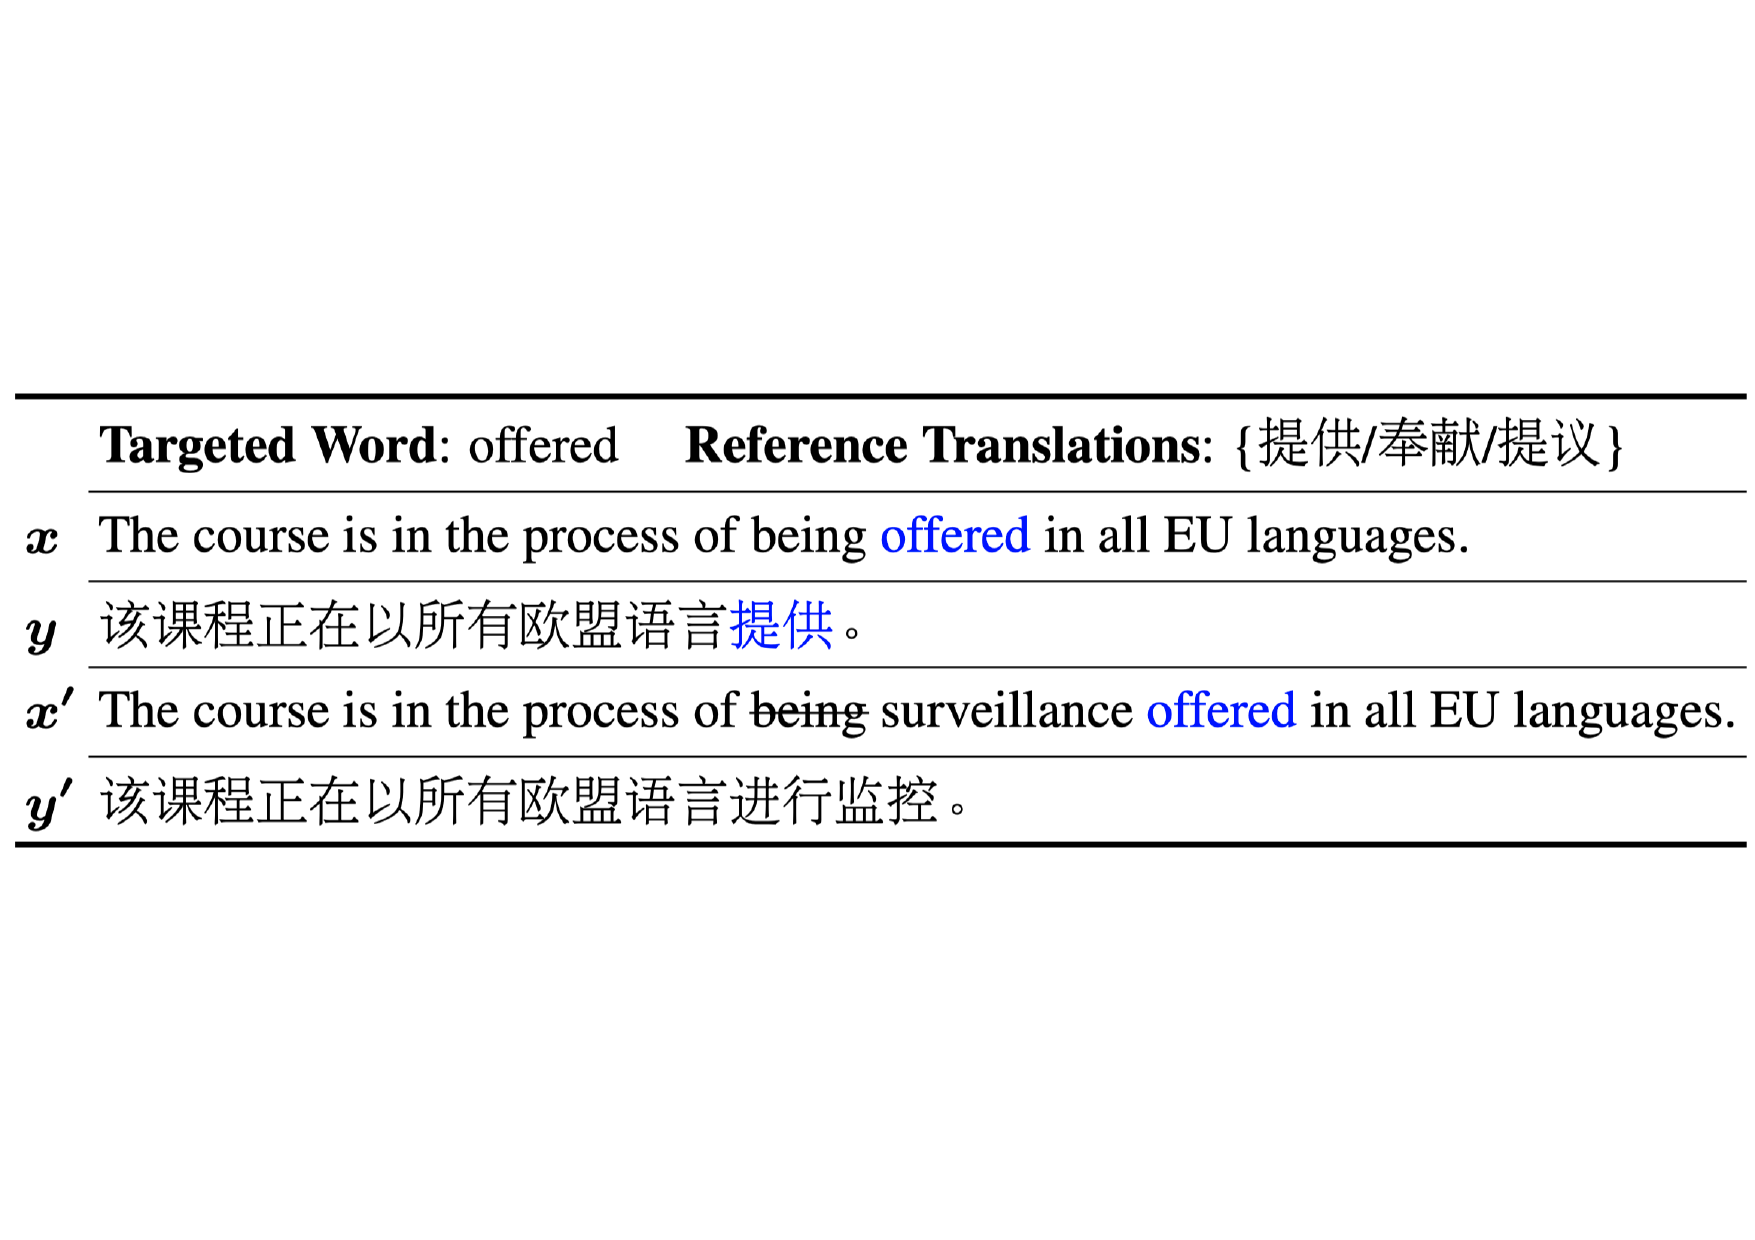}
    \caption{A case of using TWGA to attack a verb.} %The targeted word and its translation are in blue.} %Modifications are marked with orange.} 
    \label{fig:pos examples}
\end{figure}
